# Supplementary material for: Encoding information onto the charge and spin state of a paramagnetic atom using MgO tunnelling spintronics
Source: arXiv:2308.16592 source file (2025-03-14)
Supplement: Supplementary file 1 [file SI.pdf]

## Supplementary Information

Note 1: Current plume of quantum interference

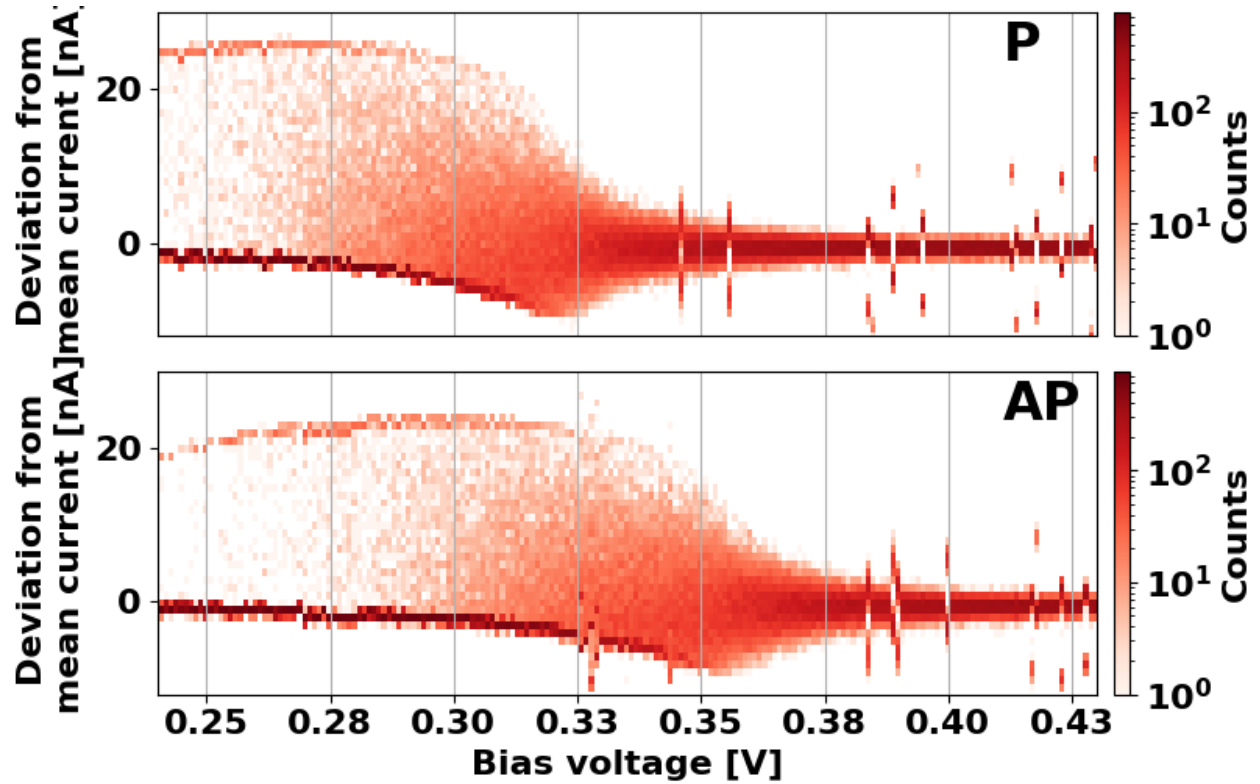

*Suppl. Fig. S1: **Zoom on the plume of quantum interference.** Bias dependence of the frequency of the deviation from the mean current. Data at  $T = 10\text{K}$  in the MTJ's P (top) and AP (bottom) states is shown. Nanojunction C5 was used. Statistics are obtained on 800 points at each bias value.*

We present in Suppl. Fig. S1 a high resolution dataset of the current distribution plume reported in Fig. 3 of the main text for the junction's P and AP states. We observe a positive 33mV bias shift of the AP dataset due to spin accumulation (see main text).

For each bias voltage we measured 800 times the junction current. The mean current is calculated and subtracted for all points inside the dataset, and finally an histogram is computed with a bin size of 1nA. The result of the histogram is represented on the Suppl. Fig. S1 by a vertical line of dots at the corresponding voltage bias, the color of a dot representing the number of counts in every bins of the histogram.

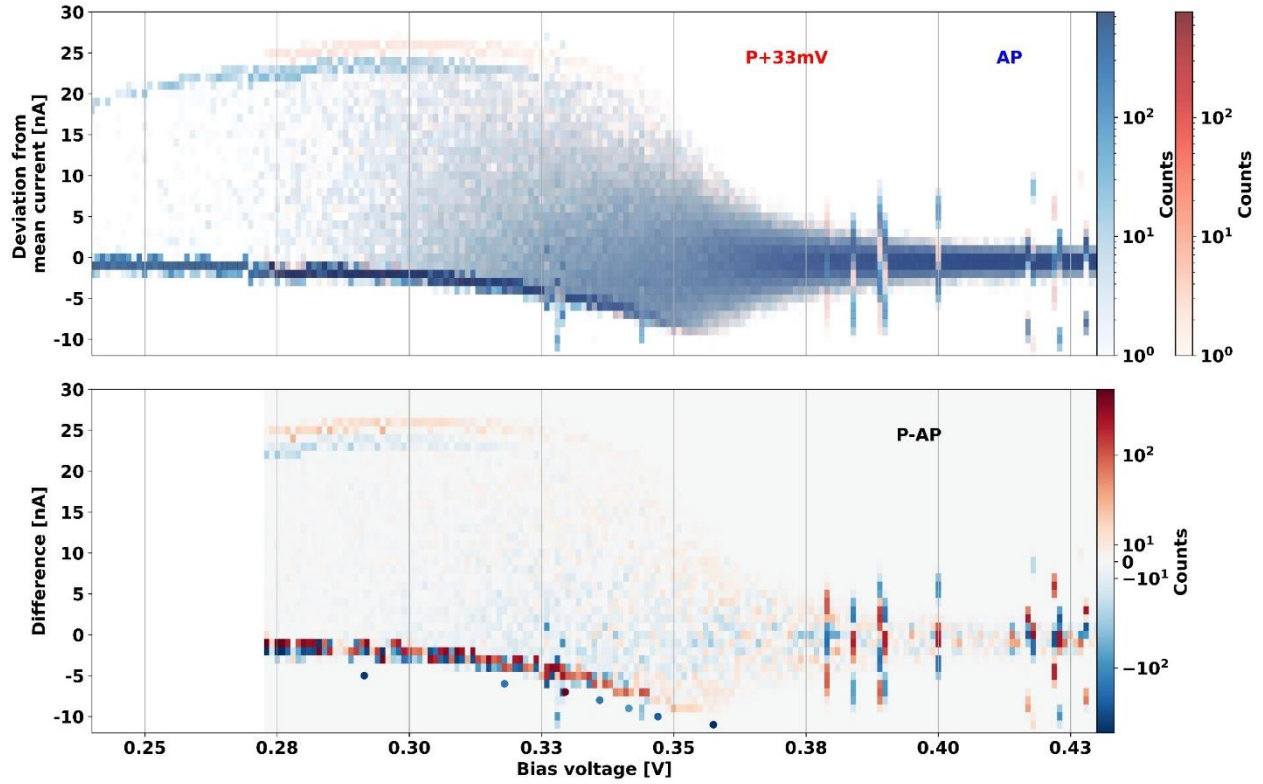

Suppl. Fig. S2: **Spintronic contrast in the plume of quantum interference.** (Top) Same data as in Suppl. Fig S. 1, but with a +33mV shift in the P data. (Bottom) Difference P-AP of the datasets of the top panel. The round dots below the lower branch represent an average of the lower branch difference data. They are centered around the range considered. These points are all blue-leaning: the lower branch is more strongly weighed in the MTJ's AP state.

To distinguish spintronic contrast, we overlap the datasets by manually removing the shift (see Fig. S2a). We note that the OFF branch (lower branch) overlaps rather well. On the other hand, the ON branch (upper branch) exhibits a different deviation from mean current in the MTJ's P and AP states. We attribute this differing deviation to a slight change in the effective potential landscape due to spin-polarized hybridization between the electrodes and the localized paramagnetic barrier states.

To further examine spintronic contrast, we then consider the difference P-AP between the datasets. The results are plotted in the bottom panel of Suppl. Fig. S2. We observe that the difference is very pronounced for the OFF branch. To confirm this trend, we've integrated this difference over several bias ranges. The position of the resulting round dots below the OFF branch represents the center of the range, while the color code shows the averaged result. Over the seven bias ranges considered, all averages of the OFF branch reveal that the OFF branch is more prevalent in the MTJ's AP state. We infer that the transport path responsible for the OFF branch is spin-polarized.

**Note 2: Spin accumulation at negative bias**

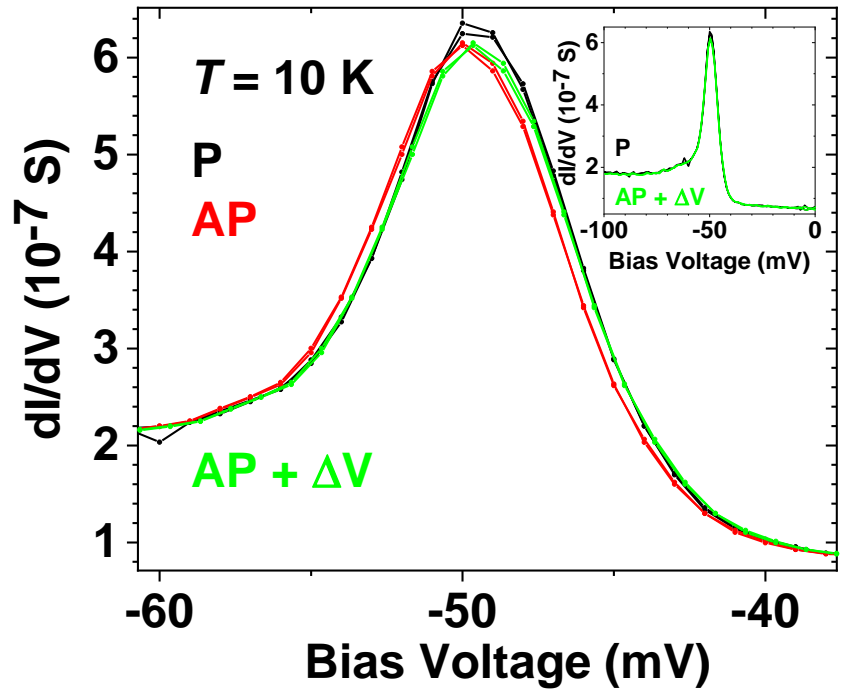

*Suppl. Fig. S3: **Spin accumulation on the sharpest Coulomb blockade peak found at  $V < 0$ .** Bias dependence of differential conductance  $dI/dV$  at  $T = 10\text{K}$  on junction G10 in the MTJ's P (black) and AP (red) states. the AP data in green was bias-shifted by  $+0.35\text{mV}$ . This shift enables a qualitatively good overlap of the conductance peak with that seen in the P data. Inset: Overview of the conductance peak in the MTJ's P state, and the bias-shifted AP data.*

In the main text, we present evidence at  $V > 0$  of a shift to higher bias values of the Coulomb blockade peaks when the MTJ's magnetic state is switched from P to AP. We now consider the case of  $V < 0$ , and focus on the Coulomb blockade peak shown in Suppl. Fig. S3. Its presence can also be switched on/off thanks to writing events  $E+$  and  $E-$ , leading to different values of TMR at that bias position (see Fig. 2 of the main text). The data of Suppl. Fig. S3 is acquired within  $-100 < V \text{ (mV)} < 0$ , i.e. below the writing events  $E-$  and  $E+$  (see inset). An excellent overlap between the P and AP data is seen for bias value below the peak. However, as the peak onset is reached, a bias shift is clearly seen. The very close agreement in the data for the forward and reverse scans underscores that the shift is not the result of trivial charging/heating effects. To qualitatively estimate the small bias shift between the P and AP data, we manually shift the AP data. A reasonable fit is found for a bias shift of  $0.35\text{mV}$ .

### Note 3: Statistics on the memristive effect

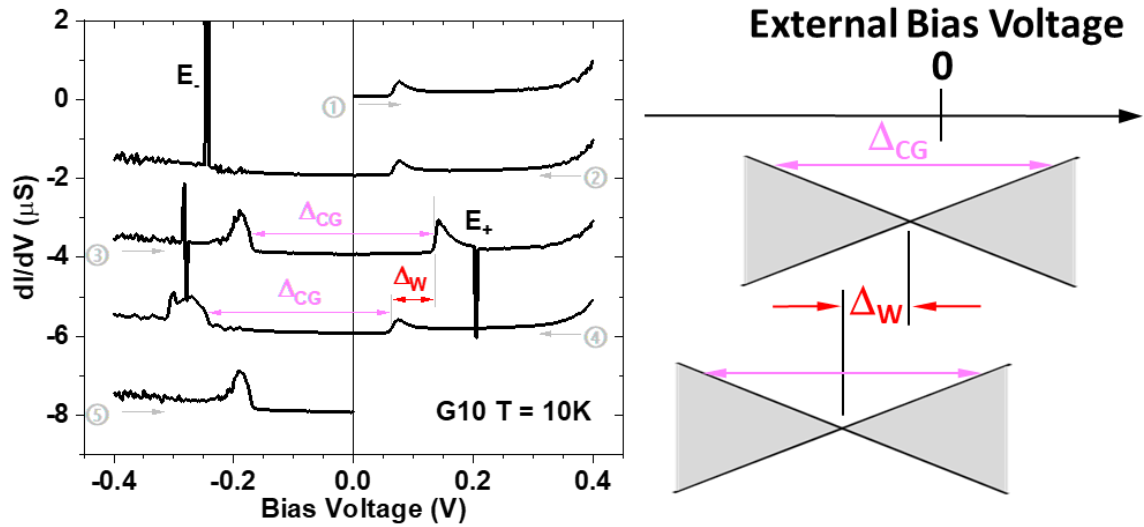

Suppl. Fig. S4: **Overview of the memristive Coulomb diamond shift.** (left) Differential conductance  $dI/dV$  vs. bias voltage on junction G10 at 10K. Successive data branches are shifted by  $2\mu S$ . The  $E_+$  and  $E_-$  writing events cause a shift  $\Delta_W=73mV$  in the constant Coulomb gap  $\Delta_{CG}=310mV$ . (Right) Proposed energy diagram of the readout QD in the two  $E_-$  and  $E_+$  states. The justification is provided in the discussion to Suppl. Fig. S8.

In the main text, we discuss how current jumps can displace the bias position of pairs of peaks associated with the Coulomb blockade diamond. In this note, we consider the statistics of this electric field-induced shift in the Coulomb diamond. To do so, we first plot an overview of the memristive Coulomb blockade effect in Suppl. Fig. S4. We observe that successive forward and reverse branches reveal a set of two conductance peaks separated by the same  $\Delta_{CG} = 310mV$ . The  $E_+$  and  $E_-$  writing events cause a shift  $\Delta_W=73mV$  in this pair of conductance peaks.

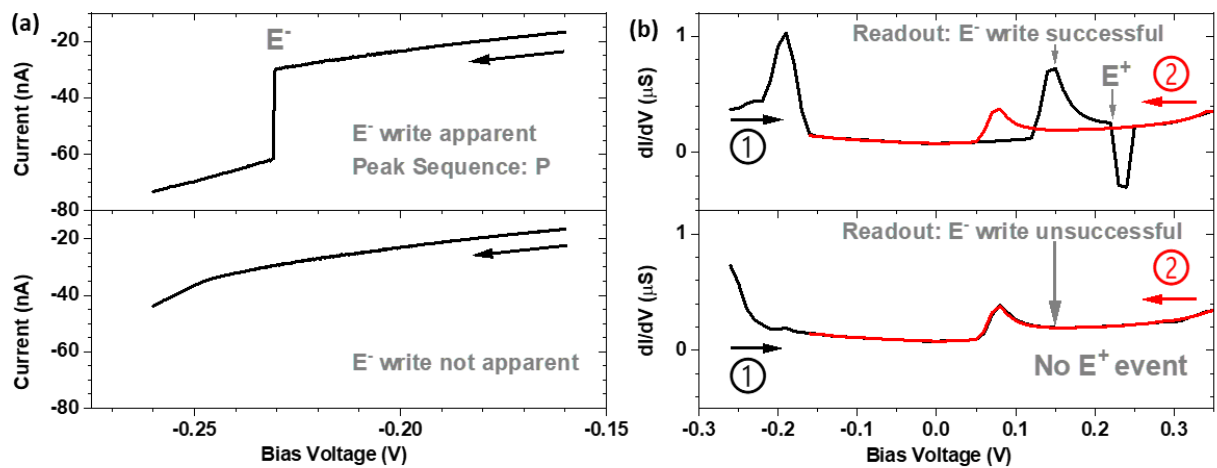

**Suppl. Fig. S5: Protocol to test junction state writing.** (a) Examples of IV traces showing E<sup>-</sup> write events that are (top) apparent, with 1 write peak observed, and (bottom) not apparent, i.e. with no write peak observed. (b) Corresponding readouts, with (top) confirmation and (bottom) information that the E<sup>-</sup> event-driven junction state was written.

To obtain statistical data on the ability to write a junction state, we undertook 1357 measurements on junction C5 at 10K. Examples of the write and read protocols are shown in Fig. S.5. In general, attempting to activate the E<sup>-</sup> write event at negative bias generates a 81% success rate in the readout at positive bias. As we explain later, this success rate would likely increase if the maximum voltage of the writing IV protocol had been increased.

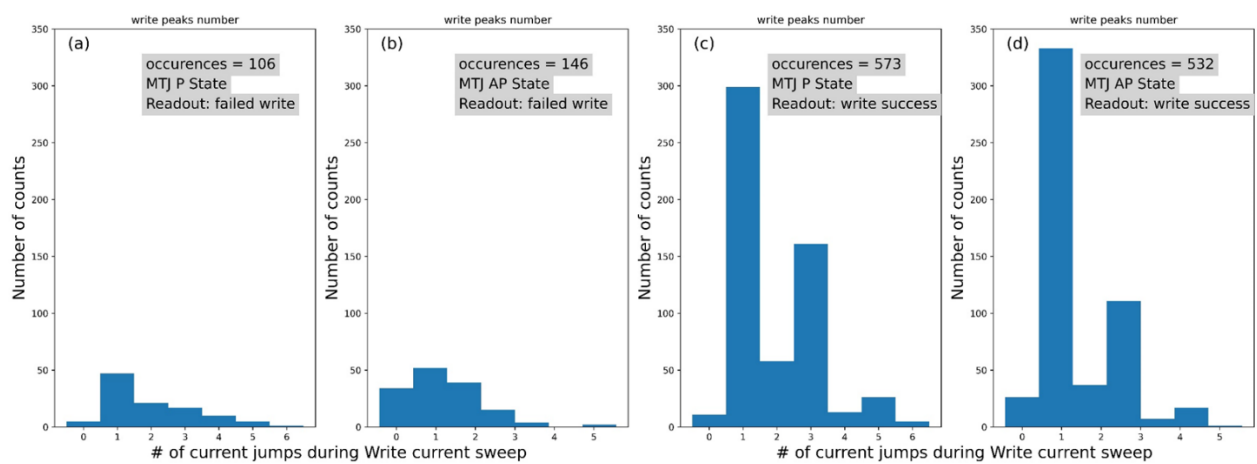

**Suppl. Fig. S6: Statistics on the success and failure to write the junction state.** The repeated protocol shown in SI Fig. S5 was used. The statistics are shown as a function of the number of current jumps during the Write current sweep.

Referring to Suppl. Fig. S6, we note that the failure to write event E- in the MTJ's P state occurs mostly for one current jump, whereas it is spread over 0-2 jumps for the AP state. There are many AP write attempts without a current jump. Furthermore, for both P and AP MTJ states, cases with an odd number of current jumps dominate even cases.

| <b>Current Jump sequence (1<sup>st</sup> ... Last)</b> | <b>Write Failed: # events</b> | <b>Write OK: # events</b> | <b>Write Success (%)</b> |
|--------------------------------------------------------|-------------------------------|---------------------------|--------------------------|
| <b>PN</b>                                              | 57                            | 93                        | 62                       |
| <b>PNPN</b>                                            | 14                            | 20                        | 59                       |
| <b>PNPNPN</b>                                          | 2                             | 2                         | 50                       |
| <b>P</b>                                               | 88                            | 548                       | 86                       |
| <b>PNP</b>                                             | 32                            | 271                       | 89                       |
| <b>PNPNP</b>                                           | 5                             | 43                        | 90                       |
| <b>PNPNPNP</b>                                         | 1                             | 4                         | 80                       |
| <b>No jump</b>                                         | 39                            | 37                        | 49                       |

*Suppl. Table S1: Statistics of write success/failure according to the sequence of absolute current increase (P) and decrease (N).*

To obtain more insight, we examine the sign of current change and current peak sequences in the entire dataset. We observe that:

- if there is a peak, the first peak is always P. This means that the first current jump is always to more negative current values.
- the sign of succeeding current peaks is always opposite, i.e. there isn't a single PP or NN sequence or subsequence in our entire dataset.
- an odd number of current jumps (i.e. ending in P) has an overall success rate of 87%. This decreases to 61% for an even number of jumps (i.e. ending in N).

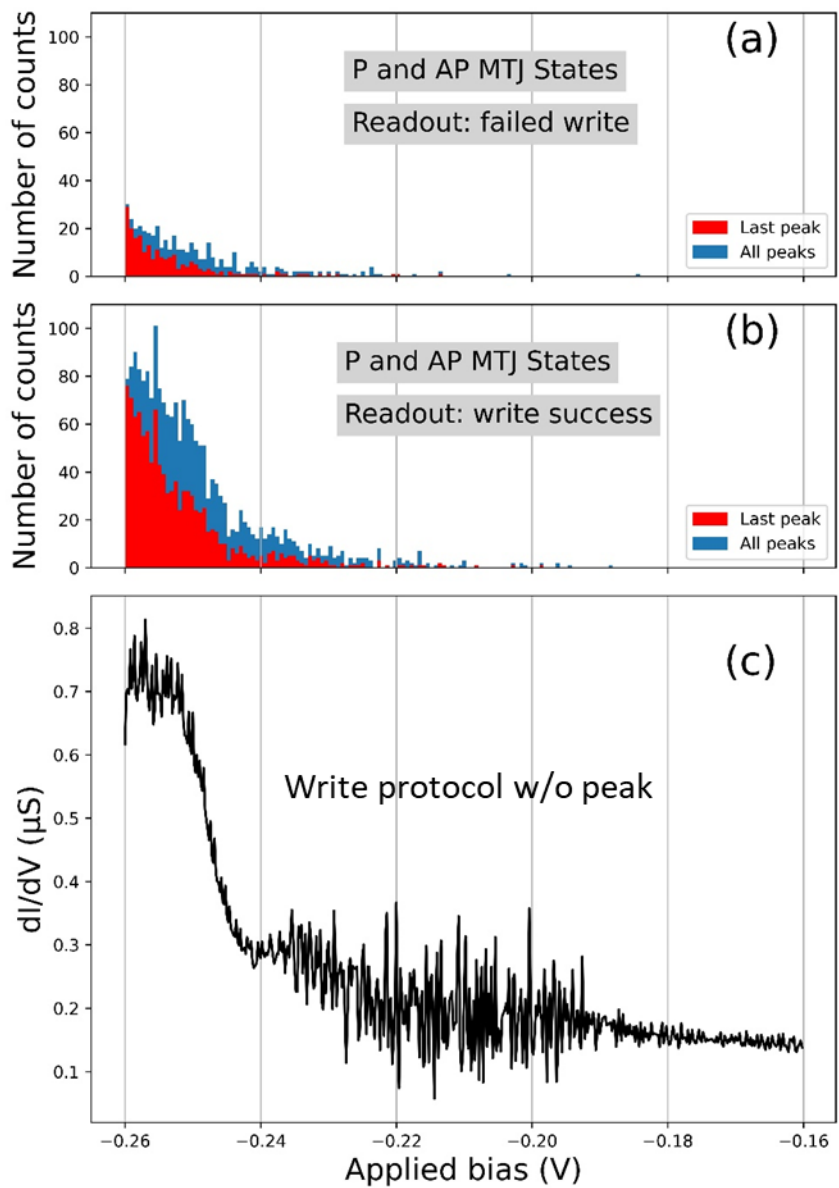

*Suppl. Fig. S7 : **Spectroscopy of current jumps.** Bias dependence of the frequency of a current jump when the writing event (a) fails and (b) succeeds. (c) Bias dependence of junction conductance when no current jump was observed. The average of 60 AP datasets is shown.*

We compare in Suppl. Fig. S7 the bias dependencies of the baseline  $dI/dV$  for the junction's  $E^+$  state (i.e. without a current jump / conductance peak), and of the current jump event frequency. We observe that

almost all current jump events occur within the bias range at which a clear conductance increase is observed. We note that the successful write events mimick most closely this dependence/amplitude, while the failed current increase events occur mainly near the peak height. Conversely, very few current jumps, whether successful or not in promoting the E- writing event, are found within the  $-0.242 < \text{Bias (V)} < -0.188$  range that exhibits transport noise. We conclude that, for this junction state, the E- writing event begins with the charging of the transport quantum dot, and not with a charging of the environmental quantum dot.

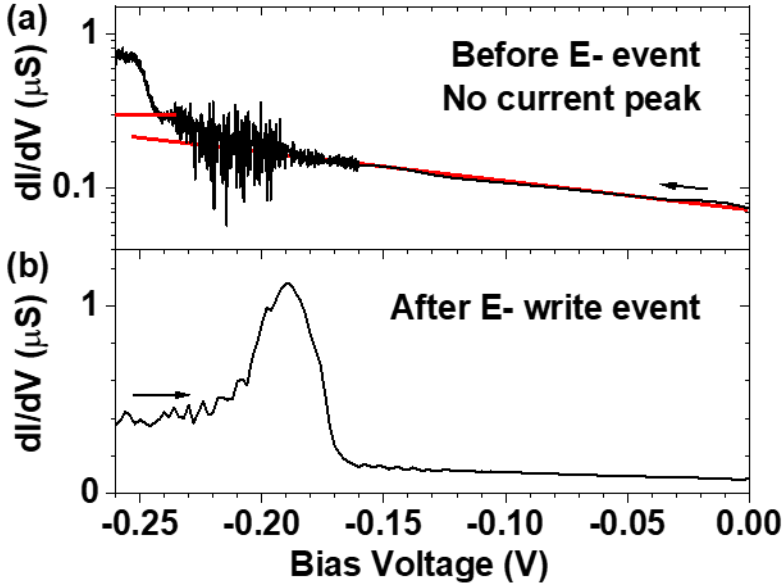

*Suppl. Fig. S8: Origin of transport noise prior to E- event. (a)  $dI/dV$  traces in  $E+$  state prior to E- event. Data with no current peak was chosen. The use of the log scale removes negative jumps. The average of 60 scans in the AP MTJ state were used. (b)  $dI/dV$  in  $E-$  state. Arrows indicate the direction of data acquisition.*

We plot in Suppl. Fig. S8(a)  $dI/dV$  traces before the E- event, for which no current peak occurs. We observe an exponential increase in junction conductance starting from  $V=0$ , up to the onset of the very noisy  $-0.242 < \text{Bias (V)} < -0.188$  range (red line). Assuming that the conductance exponential increase were to remain the same across this noise range, we see that the conductance at  $V = -0.242$  V would be half that measured (straight red line). We conclude that, in this particular junction state, the quantum interference transport between the readout quantum dot and the environmental quantum dot generates a net increase in current, i.e. that the environmental QD participates in transport through higher-order processes.

To verify that readout and environmental QDs with a fortuitously same Coulomb gap (see Suppl. Fig. S4(a)) are not simply trading roles in the E- and E+ events, we plot in panel (b) the  $dI/dV$  trace after a successful E- write event. We see that this trace's conductance peak does not have a bias range that matches that for the noise seen in panel (a). Furthermore, the two spectral features do not have the

same bias extent. This suggests that the E- and E+ events do not promote different readout QDs, but that the same QD remains as readout, but with an energy landscape that is shifted by the charging of the environmental QD (see Suppl. Fig. S4(b)). The bias extent and noise envelope of this environmental QD resembles the conductance peak of QD B, but with a +35meV energy shift.

**Note 4: Overview of the several Coulomb gaps with evolving junction state and argumentation for single-atom ‘transport’ and ‘environmental’ quantum dots**

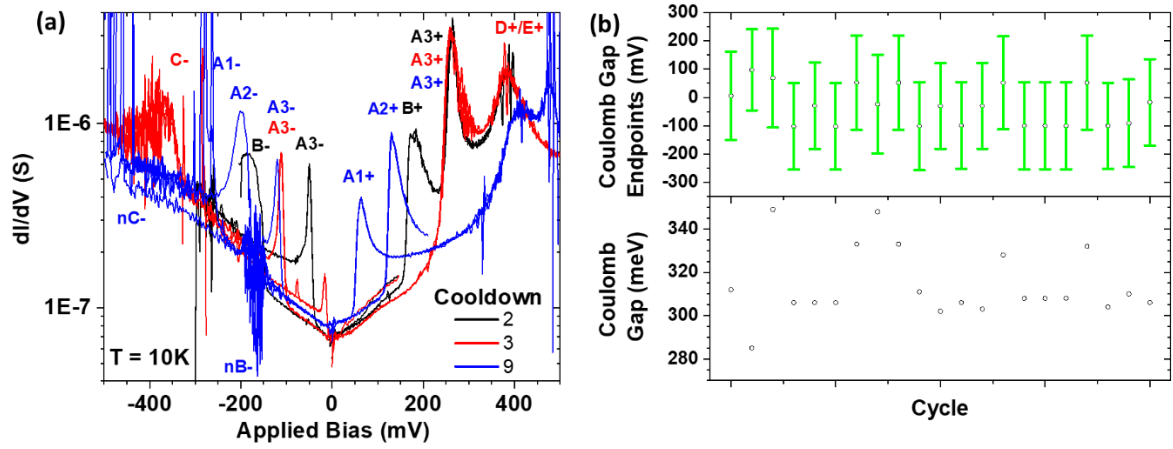

*Suppl. Fig. S9: Overview of Coulomb gap energies with evolving junction state. (a) Select  $dI/dV$  traces for three cooldowns. (b) (top) Endpoints of the Coulomb gap for select datasets deduced from the bias spacing of pairs of conductance peaks. (bottom) The resulting Coulomb energy gap of the transport atom. Junction G10 was used. The data from four cooldowns was used.*

In our datasets, we observe that heating/cooling our FeCoB/MgO/C/MgO/FeCoB junctions, and bias cycling, can alter the effective potential landscape inferred at  $T=10$  K from the current derivative. To illustrate these effects, we focus on junction G10. We plot in Suppl. Fig. S9(a) select  $dI/dV$  traces obtained after three cooldowns. We have looked for a pattern of pairs of peaks with the same energy spacing as thermal and electrical cycling were conducted. This led us to label pairs of peaks and ascribe them to the charging of a given C atom. In total we identify at least 3, and as many as 5, atoms involved in the device’s electrical response. As described in the main text, these atoms can be in the main transport path. In that case, charging the atom generates a conduction peak. Alternately, the atom in question can be tunnel coupled to a C atom that is in the transport path, and thus constitutes an ‘environmental’ atom. Following the deductions of Suppl. Fig. S9 and accompanying text, we assumed that energy motion of a pair of peaks was due to changes in the environmental charge felt by the transport atom, rather than the reattribution of ‘transport’ and ‘environmental’ roles. This logic is supported by the fairly stable energy gap between the paired peaks (see Suppl. Fig. S9(b)).

Using this labelling logic, we find for example, for cooldown #9, that pairs of conductance peaks can be attributed to the same carbon atom A, and that, in the course of IV cycling, three absolute energy positions of its Coulomb gap (see labels A1-, A2-, A3- and A1+, A2+ and A3+ in Suppl. Fig. S9(a)) relative to the MTJ electrodes' Fermi level can be tracked as the environmental charge is varied through write events E+ and E- (see main Text). Note how after an E+ writing event the pair of peaks shifts to lower absolute bias. The reverse occurs for an E- writing event. This trend in the bias shift was systematically observed, when a shift indeed occurred (see SI Note 2).

We observe additional conductance peaks at higher absolute bias voltage. In the absence of a clear trend suggesting additional charging of atom A, we surmise that these peaks correspond to additional atoms (C, D...) directly in the transport path.

Comparing these cooldowns, we observe that the peak of a  $dI/dV$  in one cooldown can spectrally correspond to noise for another cooldown. The best example is, at  $V \sim 190\text{mV}$ , that of peak B- in cooldown 2 (black), and of the corresponding noise nB- in cooldown 9 (blue). We infer that atom B is present in the transport path in cooldown 2, but becomes an environmental atom in cooldown 9. This also explains the absence of peaks B- and B+ in cooldowns 3 and 9.

We also observe that, in the junction state defined by cooldowns 3 and 9, the writing event E+ occurs just as the spectral window B+ corresponding to environmental atom B is reached with increasing positive bias around +150 mV. This illustrates the role that the charge state of environmental atom has in the junction write process (see main text).

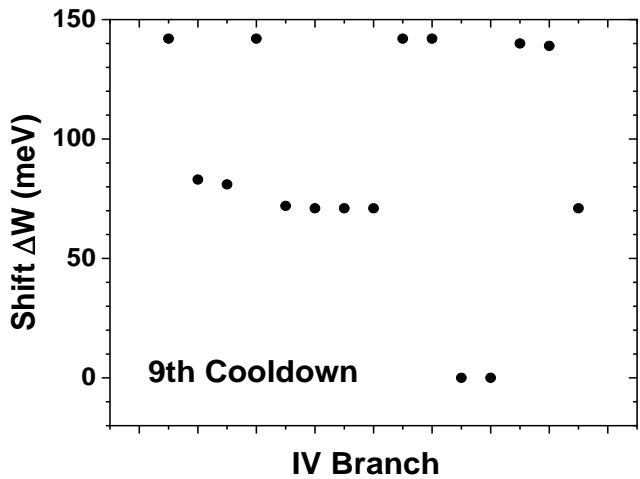

transport role, However, those junction states promoted only two pairs of peaks. We present in Suppl. Fig. S10 the energy shift  $\Delta W$  data in junction cooldown 9 arising from the presence of 3 pairs of peaks due to transport atom A. Aside from the trivial  $\Delta W=0$  points due to write failure (see SI Note 2), DW takes on multiple values of 70-80meV. Here, we make the reasonable assumption that the charge of an environmental atom can only change by 1 electron, which implies that several environmental atoms can be charged during a write event.

#### Note 5: Estimation of the impurities sizes and distances

Let us approximate the impurity involved in transport as a sphere of radius  $r$ , located at a distance  $d$  from the lower electrode, with interelectrode spacing  $l$ . In the far-field limit, the capacitance  $C$  is given in Ref. 1 and reads:

$$C = \frac{4\pi\epsilon\epsilon_0 r}{1 + \left(\psi^{(0)}\left(\frac{d}{l}\right) + \psi^{(0)}\left(1 - \frac{d}{l}\right) + 2\gamma\right) \frac{r}{2l}},$$

where  $\psi^{(0)}$  is the polygamma function. Using the relation between the capacitance and the charging energy  $E_C = e^2/2C = e\Delta_{CG}$ , we obtain the radius of the impurity

$$r = \frac{l}{8\pi\epsilon\epsilon_0 \Delta_{CG}/e + 5/3}$$

where  $\frac{1}{2}(\psi^{(0)}(d/l) + \psi^{(0)}(1 - d/l) + 2\gamma) \approx -5/3$  with  $d = 1$  nm and  $l = 3$  nm as approximated from the experimental design of the stack. Taking  $\epsilon = 9$  for the relative permittivity of MgO according to Ref. 2, we obtain  $r = 0.2$  nm. This shows that the impurities involved in the transport are of atomic sizes and should indeed correspond to single carbon atoms or dimers trapped inside the MgO lattice.

Let us now approximate both the transport and environmental quantum dots as two spheres of radius  $r$ , separated by a distance  $d$ . The capacitance  $C$  of the system is approximately given by:

$$C = \frac{2\pi\epsilon_0\epsilon r}{1 - \frac{r}{d-r}}$$

According to the observed shift  $\Delta_W = 70$  mV which shall be due to the change of charge of one environmental quantum dot by a quantum of elementary charge, we should then write:

$$e = C\Delta_W.$$

which leads to the distance between the dots:

$$d = r \left( 1 + \frac{1}{1 - \frac{2\pi\epsilon_0\epsilon r \Delta_W}{e}} \right).$$

With  $r = 0.2$  nm as estimated above; we obtain the following approximation:

$$d \approx 2r ,$$

such as  $d = 0.4$  nm. We thus find that the distance between the transport quantum dots and the environmental charging species is of the order of the diameter of the dots, so the control dot should be a second, third or forth neighboring site of the transport dot in the MgO lattice. This estimation confirms that we are indeed observing the interaction of a reduced number of atomic formations closely packed inside the MgO barrier which are producing single-electron effects.

#### Note 6: Other junctions

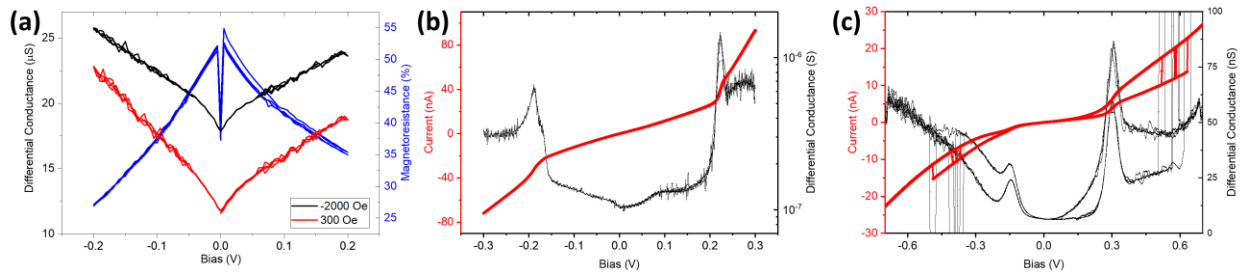

**Suppl. Fig. S11: Magnetotransport experiments on other junctions.** (a) Differential Conductance for the P (black) and AP (red) states and TMR (blue) plots at 10 K for junction F10. (b) and (c) Intensity-potential (black) and differential conductance (red) plots at 10 K and -2000 Oe for junctions B11 and B5 respectively.

Magnetoresistive properties have also been measured on several of these junctions, of the same kind as G10 and C5 presented in the main text. SI Fig.S11(a) shows that the electrical intensity of the junction F10 differs between the P and the AP configurations of the electrodes. This results in an apparent magnetoresistance of up to 60% that is maximal around 0. The conductance plot features two singular characteristics. First, the V-shaped spike around 0 mV, referred as the Zero-Bias anomaly (ZBA) [3-5], may indicate that an impurity state close to the Fermi level is located inside the MgO barrier [6]. This ZBA seems more pronounced in the P state than in the AP state as the deviation from linearity is more present at -2000 Oe in SI Fig.S11(a). Then, the noise visible in the linear part of the conductance, above 50 mV and below 50 mV should indicate the presence of two or more states close in energy which would result in several interfering nanotransport paths. An asymmetry is also observed in this figure: at negative bias the conductance is higher than at positive bias, in particular in the AP state which suggests that a structural asymmetry renders the electrodes nonequivalent. The drop in the junction resistance with increasing bias voltage is greater for antiparallel alignment of the magnetic electrodes than for parallel alignment which has been accounted for by spin excitations localized at the interfaces between the electrodes and the tunnel barrier [3].

Of the 58 devices which have been tested, four other junctions displayed memristive behaviors, similar to G10 and C5, containing branch jumps and conductance peaks (see Figure SI Fig.S11(c)) which suggests the potential reproducibility of this phenomenon. Five other junctions also presented non-linear intensity-potential characteristics (see SI Fig.S11(b)) translating into sharp conductance peaks, but without branch jumps, looking more like standard MgO junctions without Carbon inside, but with a lower magnetoresistance.

#### Note 7: Memristance and temperature dependance

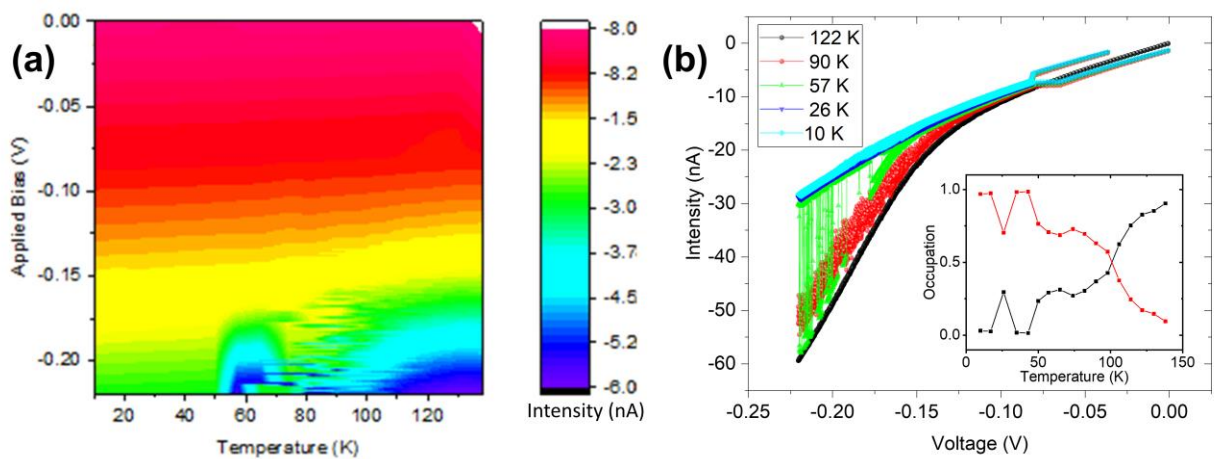

Suppl. Fig. S12: **Temperature dependance of the memristive behavior.** (a) Color plot of the current as a function of the temperature and applied bias for junction G10. (b) Intensity-Voltage characteristic of junction G10 recorded at five different temperatures. Inset: occupation probability of the low (in red) and high (in black) absolute intensity branches as a function of temperature.

## Note 8: Magnetoresistance

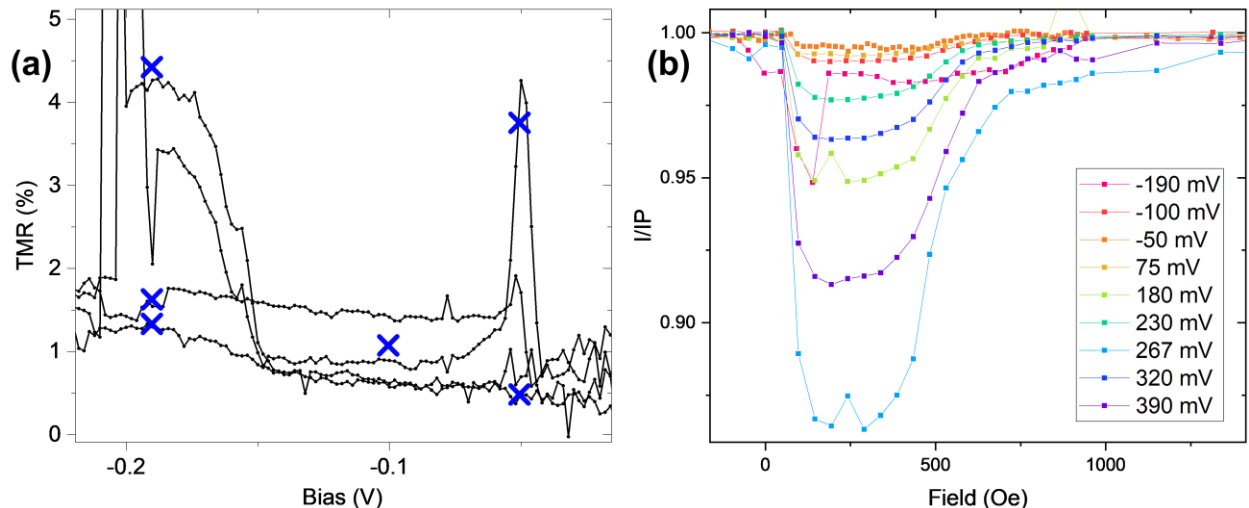

Suppl. Fig. S13: **Magnetoresistance.** (a) Plot of the tunnel magnetoresistance as a function of the bias calculated from the intensity-voltage characteristic in the P and AP states of junction G10. The blue crosses represent points that have been confirmed by  $I(H)$  experiments. The TMR enhancement due to the different memristive Coulomb blockade peaks can be observed. (b) Relative intensity compared to the P state as a function of the external field for different applied bias obtained from junction G10.

- [1] A. M. Drews, M. Kowalik, and K. J. M. Bishop, "Charge and force on a conductive sphere between two parallel electrodes: A Stokesian dynamics approach," *Journal of Applied Physics* 116, 074903 (2014).
- [2] D. R. Lide, G. Baysinger, S. Chemistry, L. I. Berger, R. N. Goldberg, and H. V. Kehiaian, "CRC Handbook of Chemistry and Physics".
- [3] S. Zhang, P. M. Levy, A. C. Marley, and S. S. P. Parkin, "Quenching of Magnetoresistance by Hot Electrons in Magnetic Tunnel Junctions," *Physical Review Letters* 79, 3744–3747 (1997).
- [4] A. F. G. Wyatt, "Anomalous Densities of States in Normal Tantalum and Niobium," *Physical Review Letters* 13, 401–404 (1964).
- [5] J. A. Appelbaum and L. Y. L. Shen, "Zero-Bias-Conductance Peak Anomaly of Ta-I-Al Tunnel Junctions at 0.3 K and 90 kG," *Physical Review B* 5, 544–553 (1972).
- [6] G.-X. Miao, M. Münzenberg, and J. S. Moodera, "Tunneling path toward spintronics," *Reports on Progress in Physics* 74, 036501 (2011).
- [7] <https://lmfit.github.io/lmfit-py/>
